# Supplementary material for: Provable and Efficient Continual Representation Learning
Source: arXiv:2203.02026 source file (2022-11-07)
Supplement: Supplementary file 1 [file proof_bc.tex]

\section{Appendix B: Proof of Theorem \ref{cl thm}}

%In what follows, we consider a generalization of the scenario where tasks arrive one by one. Specifically, let us assume that each task is composed of multiple sub-tasks. We are given a new task with samples $\Sc=(\Sc_t)_{t=1}^\Tn$ composed of $\Tn$ new tasks. These subtasks are represented by datasets $\Sc_t=(\x_{ti},y_{ti})_{i=1}^N$ each drawn i.i.d. from distributions $\Dc_t$ for $t\in[\Tn]$. Our goal is building hypothesis $(f_t)_{t=1}^{\Tn}$ for these new sub-tasks with small sample size $N$ while leveraging $\bPf$.

In this section, we prove our main theoretical result Theorem~\ref{cl thm}.
% \Lc(\hhb,&\hat{\phi})\leq \Lco_{\pfh}+ \Gamma\sqrt{\frac{\ordet{T\cc{\Hb}+\cc{\bPn}+\tau}}{TN}},\nn\\
% &\leq \Lco+\MM+\Gamma\sqrt{\frac{\ordet{T\cc{\Hb}+\cc{\bPn}+\tau}}{TN}}\nonumber.\nonumber

\begin{proof} To be start, let $\Hb_\eps$ and $\bPhi_{\text{NEW},\eps}$ be $\eps$-covers of $\Hb$ and $\bPn$ and define $\vct\Fc=\Hb_\eps^T\times\bPhi_{\text{NEW},\eps}$. Following the Def.~\ref{def:cov} we have 
\begin{align}
    \log|\vct\Fc|\leq D ~~~\text{where}~~~\red{D:=(T\Cc(\Hb)+\Cc(\bPn))\log((\BC/\eps))}. \nn
\end{align}
Set $t=\sqrt{\frac{D+\tau}{cNT}}$ where $c>$ is an absolute constant. Since loss function $\ell(\cdot)$ is bounded in $[0,1]$, then following Hoeffding inequality we have
\begin{align}
    \P(|\Lc(\hhb,\hat{\phi})- \Lco_{\pfh}|\geq t)&\leq2|\vct\Fc|e^{-cNTt^2}, \nn\\
    &\leq2|\vct\Fc|e^{-D-\tau}, \nn\\
    &\leq2e^{-\tau}. \label{prob}
\end{align}
Now consider about the task-averaged risk perturbation introduce by covered set. Let $\pn,\pn'\in\bPn,\bPhi_{\text{NEW},\eps}$ and $h,h'\in\Hb,\Hb_{\eps}$ be $L$-Lipschitz functions (in Euclidean distance). Then $\phi:=\pn+\pf$ and $\phi':=\pn'+\pf$ also satisfy $L$-Lipschitz constraint. %Consider bounded input $\x$, and set $R=\max(L,1)\tn{\x}$
\begin{align}
    \Lc(\hb,\phi)- \Lc(\hb',\phi')&\leq|\Lc(\hb,\phi)- \Lc(\hb',\phi')|, \nn\\
    &\leq \sup_{t\in[T]}|\Lc_{\Sc_t}(h_t,\phi)-\Lc(h_t',\phi')|, \nn\\
    &\leq \sup_{t\in[T], i\in[N]}|\ell(y_{ti},h_t\circ\phi(\x_{ti}))-\ell(y_{ti},h_t'\circ\phi'(\x_{ti}))|, \nn \\
    &\leq \Gamma\sup_{t\in[T], i\in[N]}|h_t\circ\phi(\x_{ti})-h_t'\circ\phi'(\x_{ti})|, \nn\\
    &\leq\Gamma\sup_{t\in[T], i\in[N]}|h_t\circ\phi(\x_{ti})-h_t\circ\phi'(\x_{ti})|+|h_t\circ\phi'(\x_{ti})-h_t'\circ\phi'(\x_{ti})|, \nn\\
    &\leq \Gamma (L+1)\eps. \label{pert}
\end{align}
Combine results from \ref{prob} and \ref{pert} by setting $\eps=$, then we find that with probability at least $1-2e^{-\tau}$
\begin{align}
    \Lc(\hhb,\hat{\phi})- \Lco_{\pfh}\leq\Gamma(L+1)\eps+\sqrt{\frac{D+\tau}{cNT}}\nn.
\end{align}
\end{proof}
