# Supplementary material for: Provable and Efficient Continual Representation Learning
Source: arXiv:2203.02026 source file (2022-11-07)
Supplement: Supplementary file 2 [file appendix.tex]

\newpage
\section{Appendix}
\subsection{Channel Pruning}
To prune channel effectively and iteratively, we introduce channel mask in continuous value ($\Mc_l\in\R^{n_l}, l\in [L]$) to induce sparsity where $L$ is layer count each with $n_l$ channels/neurons. In our experiments, inspired by \cite{liu2017learning} we adopt BatchNorm layers and extract their weights as masks. Then we have
\begin{align*}
	\x_l=(\Mc_l\cdot \text{norm}(\text{conv}(\x_{l-1})))_+,~~\text{norm}(\z)=\frac{\z-\mu_\z}{\sqrt{\sigma_\z^2+\epsilon}}
\end{align*}
where $\x_l$ is the output feature of $l^{th}$ layer and $\Mc_l$ is trainable masked weights of BN layer.

Given a single task, structure pruning is trying to find and remove insignificant channels/neurons without hurting performance. To achieve this goal, we propose a FLOP-base sparsity regularization
\begin{align*}
	\Rc(\Mc)&=\sum_{l\in [L]}\lambda_l\|\Mc_l\|_1\\
	&=\sum_{l\in[L]}\frac{g(\text{FLOP}_l(\Mc))}{\sum_{j\in[L]}g(\text{FLOP}_j(\Mc))}\|\Mc_l\|_1
\end{align*}
where $\lambda_l$, $\Mc_l$ and $\text{FLOP}_l(\cdot)$ denote regularization parameter, channel mask and FLOP calculation function of $l^{th}$ layer. We apply $\ell_1$-norm to achieve sparsity, since it enforces unimportant elements to zeros. $g(\cdot)$ is monotonically increasing function used to calculate $\lambda_l$ automatically.
In deep neural network, different layer has different FLOPs load corresponding to its input/output feature size and operations. Therefore, it is unfair to use global regularization parameters. We adopt layerwise regularization parameter $\lambda_l$ and relate it to FLOPs load. Our goal is to push layers with more FLOPs sparser. Results show that this approach achieves good results especially when the network is pruned to very sparse. In our experiments, we use $g(x)=\sqrt{x}$.

\begin{table}[t]
    \small
    \caption{\small{Continual learning results}}
    \centering
    \begin{tabular}{lcc}
    \midrule
    & RotatedMNIST & PermutedMNIST\\
    \midrule
    ESPN-0.2 &97.21$\pm$0.007 95.78$\pm$0.015\\
    PackNet &95.66$\pm$0.014 & 92.88$\pm$0.024\\
    Individual-0.2&95.48$\pm$0.370 & 95.36$\pm$0.303\\
    Individual-1 &97.36$\pm$0.149 & 97.31$\pm$0.107\\
    \midrule
    \end{tabular}\label{MNISTtable}
\end{table}
